# Supplementary material for: Intensities of the hydrogen Balmer lines of solar-like stars revealed by the LAMOST spectroscopic surveys
Source: arXiv:2408.01975 source file (2024-08-04)
Supplement: Supplementary file 1 [file supplementary_information.pdf]

# Intensities of the hydrogen Balmer lines of solar-like stars revealed by the LAMOST spectroscopic surveys

Han He[1,2]

[1]National Astronomical Observatories, Chinese Academy of Sciences, Beijing, 100101, China email: hehan@nao.cas.cn
[2]University of Chinese Academy of Sciences, Beijing, 100049, China

## Supplementary Methods

### Signal-to-noise ratios of the LRS and MRS spectra of solar-like stars employed in this work

Supplementary Figure S1 shows the scatter plot of S/N$_r$ vs. S/N$_g$ for the LRS spectral sample of solar-like stars (panel (a)) and the scatter plot of S/N$_R$ vs. S/N$_B$ for the MRS spectral sample of solar-like stars (panel (b)) employed in this work. It can be seen from Supplementary Fig. S1 that the data points are roughly distributed along the $10 : 7$ line for both the LRS and MRS spectral samples of solar-like stars, which is utilized to assist in determining the thresholds of the signal-to-noise ratios for selecting the high-S/N LRS and MRS spectra employed in this work. The S/N thresholds can be seen in the lower left corner of the plots in Supplementary Fig. S1. The data of the signal-to-noise ratios of the LRS and MRS spectral samples are included in the dataset of this paper (see Supplementary Note and Supplementary Tables S1 and S2).

### Stellar atmospheric parameters of the LRS and MRS data for the stellar source sample of solar-like stars employed in this work

For the stellar sources observed by both the LRS and MRS, the stellar atmospheric parameters ($T_{\mathrm{eff}}$, $\log g$, and [Fe/H]) determined from both the LRS and MRS data are available. Supplementary Figures S2a–S2c (top row of Supplementary Fig. S2) show the correlation diagrams of the stellar atmospheric parameters determined from the LRS and MRS data for

the stellar source sample of solar-like stars employed in this work; Supplementary Figures S2d–S2f (bottom row of Supplementary Fig. S2) compare the distributions of the stellar parameter uncertainties of the LRS and MRS data. The data of the stellar atmospheric parameters and their uncertainties of the co-source LRS and MRS spectral samples are included in the dataset of this paper (see Supplementary Note and Supplementary Tables S1 and S2). If a stellar source was observed multiple times by the LRS or MRS, the medians of the stellar parameters of the multiple observations are used in the analysis.

It can be seen from Supplementary Figs. S2a–S2c that the stellar atmospheric parameter values of the LRS and MRS data are generally consistent with each other. Supplementary Figures S2d–S2f show that the uncertainties of the stellar atmospheric parameters ($\delta T_{\rm eff}$, $\delta \log g$, and $\delta$[Fe/H]) of the LRS and MRS data are at the similar level, but the trailing of the uncertainty distributions of the MRS data is longer than that of the LRS data; considering this issue, the stellar parameter values determined from the LRS data are used in the evaluation of the absolute flux indexes of the Balmer lines as well as in the analysis of the index distributions. It can also be seen from Supplementary Fig. S2d that the peak position of the $\delta T_{\rm eff}$ distributions of the LRS and MRS data is at about 25 K; the span of $T_{\rm eff}$ adopted in this work for the solar-like spectral sample ($\pm$75 K) is $\pm$3 times of this value. The peak positions of the $\delta \log g$, and $\delta$[Fe/H] distributions are at about 0.03 dex and 0.02 dex, respectively, as shown in Figs. S2e and S2f.

# Supplementary Note

## Dataset of this paper

The dataset of this paper consists of three catalogs of the data of the Balmer line indexes of solar-like stars obtained in this work based on the LAMOST spectroscopic surveys: the LRS spectral catalog, the MRS spectral catalog, and the stellar source catalog (corresponding to LRS spectral sample, MRS spectral sample, and stellar source sample described in the main text of the paper, respectively). These catalogs are stored as three CSV-format data files. The columns contained in the catalogs are listed and described in Supplementary Tables S1, S2, and S3, respectively; the CSV file names of the catalogs are given in the footnotes of Supplementary Tables S1–S3. The dataset is available online at https://doi.org/10.5281/zenodo.10848180.

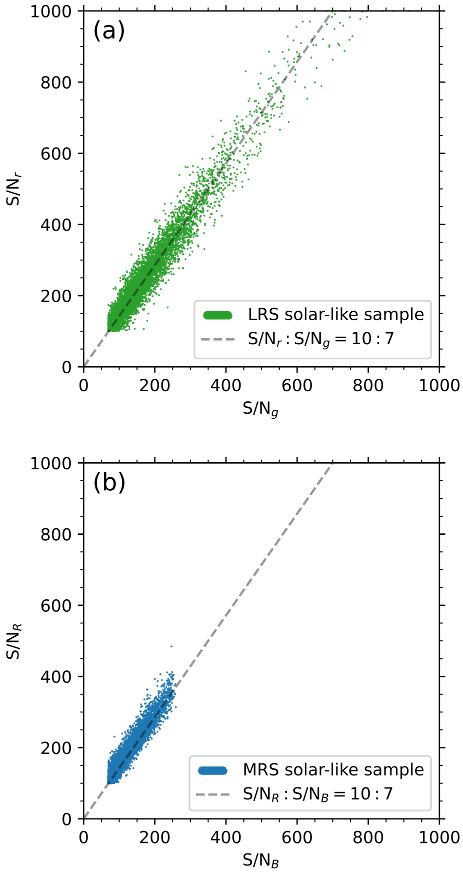


Supplementary Figure S1: (a) Scatter plots of S/N$_r$ vs. S/N$_g$ for the LRS spectral sample of solar-like stars employed in this work. (b) Scatter plots of S/N$_R$ vs. S/N$_B$ for the MRS spectral sample of solar-like stars employed in this work. The 10 : 7 line (dashed line) is displayed in the plots for reference. The S/N thresholds used for selecting the high-S/N LRS and MRS spectra can be seen in the lower left corner of the plots.

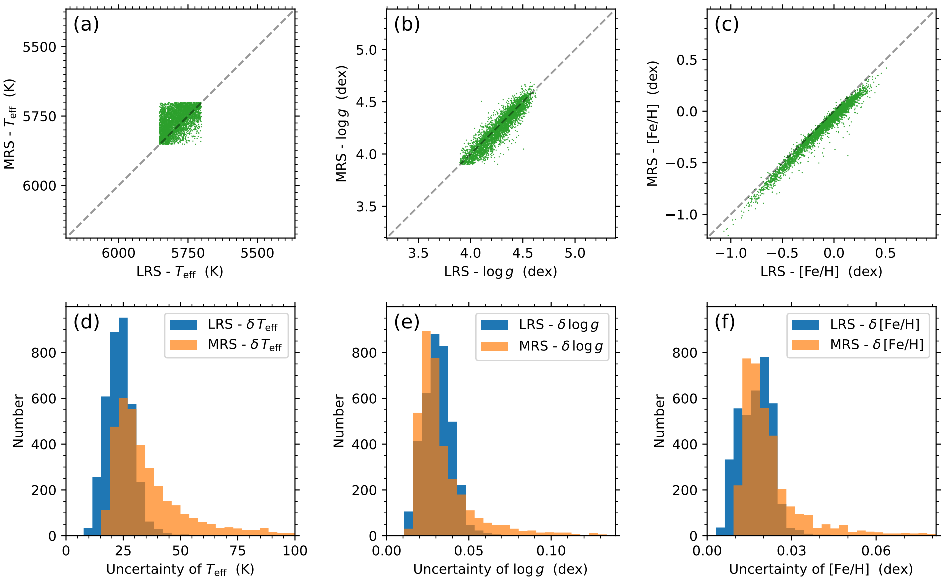


Supplementary Figure S2: (a–c) Diagram illustrating the correlations between the stellar atmospheric parameters ($T_{\rm eff}$, $\log g$, and [Fe/H]) determined from the LRS and MRS data for the stellar source sample of solar-like stars employed in this work. The 1 : 1 line (dashed line) is displayed for reference. (d–f) Distribution histograms of the uncertainties of the stellar atmospheric parameters of the LRS and MRS data.

Supplementary Table S1: Columns contained in the LRS spectral catalog.

| Column Name | Unit | Description |
|---|---|---|
| obsid | | unique LAMOST observation identifier of LRS |
| obsdate | | date of LRS observation (UTC) |
| uid | | unique LAMOST source identifier |
| ra | degree | right ascension of stellar source in LRS catalogs |
| dec | degree | declination of stellar source in LRS catalogs |
| sn_g | | LRS $g$-band signal-to-noise ratio (S/N$_g$) |
| sn_r | | LRS $r$-band signal-to-noise ratio (S/N$_r$) |
| teff | K | stellar effective temperature ($T_{\rm eff}$) determined by the LASP from LRS data |
| teff_err | K | uncertainty of $T_{\rm eff}$ |
| logg | dex | stellar surface gravity ($\log g$) determined by the LASP from LRS data |
| logg_err | dex | uncertainty of $\log g$ |
| feh | dex | stellar metallicity ([Fe/H]) determined by the LASP from LRS data |
| feh_err | dex | uncertainty of [Fe/H] |
| rv | km/s | radial velocity determined by the LASP from LRS data |
| rv_err | km/s | uncertainty of radial velocity |
| L_halpha | | H$\alpha$ activity index of LRS data ($L_{\rm H\alpha}$) |
| L_halpha_err | | uncertainty of $L_{\rm H\alpha}$ |
| L_hbeta | | H$\beta$ activity index of LRS data ($L_{\rm H\beta}$) |
| L_hbeta_err | | uncertainty of $L_{\rm H\beta}$ |
| L_hgamma | | H$\gamma$ activity index of LRS data ($L_{\rm H\gamma}$) |
| L_hgamma_err | | uncertainty of $L_{\rm H\gamma}$ |
| L_hdelta | | H$\delta$ activity index of LRS data ($L_{\rm H\delta}$) |
| L_hdelta_err | | uncertainty of $L_{\rm H\delta}$ |

Note:
(1) Catalog is stored as Balmer_line_indexes_LRS_spectral_catalog_LAMOST_DR9.csv in the online dataset.
(2) Observational and spectroscopic parameters are from LAMOST DR9 v2.0.
(3) Unavailable values are marked as −9999.0.

Supplementary Table S2: Columns contained in the MRS spectral catalog.

| Column | Unit | Description |
|---|---|---|
| obsid | | unique LAMOST observation identifier of MRS |
| obsdate | | date of MRS observation (UTC) |
| uid | | unique LAMOST source identifier |
| ra | degree | right ascension of stellar source in MRS catalogs |
| dec | degree | declination of stellar source in MRS catalogs |
| sn_B | | MRS blue-band signal-to-noise ratio (S/N$_B$) |
| sn_R | | MRS red-band signal-to-noise ratio (S/N$_R$) |
| teff | K | stellar effective temperature ($T_{\rm eff}$) determined by the LASP from MRS data |
| teff_err | K | uncertainty of $T_{\rm eff}$ |
| logg | dex | stellar surface gravity ($\log g$) determined by the LASP from MRS data |
| logg_err | dex | uncertainty of $\log g$ |
| feh | dex | stellar metallicity ([Fe/H]) determined by the LASP from MRS data |
| feh_err | dex | uncertainty of [Fe/H] |
| rv_r0 | km/s | radial velocity determined from the red band data of MRS |
| rv_r0_err | km/s | uncertainty of radial velocity |
| M_halpha | | H$\alpha$ activity index of MRS data ($M_{\rm H\alpha}$) |
| M_halpha_err | | uncertainty of $M_{\rm H\alpha}$ |

Note:
(1) Catalog is stored as Balmer_line_indexes_MRS_spectral_catalog_LAMOST_DR9.csv in the online dataset.
(2) Observational and spectroscopic parameters are from LAMOST DR9 v2.0.
(3) Unavailable values are marked as −9999.0.

Supplementary Table S3: Columns contained in the stellar source catalog.

| Column Name | Unit | Description |
|---|---|---|
| `uid` | | unique LAMOST source identifier |
| `ra` | degree | right ascension of stellar source from LRS catalogs |
| `dec` | degree | declination of stellar source from LRS catalogs |
| `teff` | K | stellar effective temperature ($T_{\rm eff}$) from LRS catalogs |
| `teff_err` | K | uncertainty of $T_{\rm eff}$ |
| `logg` | dex | stellar surface gravity ($\log g$) from LRS catalogs |
| `logg_err` | dex | uncertainty of $\log g$ |
| `feh` | dex | stellar metallicity ([Fe/H]) from LRS catalogs |
| `feh_err` | dex | uncertainty of [Fe/H] |
| `L_halpha` | | H$\alpha$ activity index of LRS data ($L_{\rm H\alpha}$) |
| `L_halpha_err` | | uncertainty of $L_{\rm H\alpha}$ |
| `L_hbeta` | | H$\beta$ activity index of LRS data ($L_{\rm H\beta}$) |
| `L_hbeta_err` | | uncertainty of $L_{\rm H\beta}$ |
| `L_hgamma` | | H$\gamma$ activity index of LRS data ($L_{\rm H\gamma}$) |
| `L_hgamma_err` | | uncertainty of $L_{\rm H\gamma}$ |
| `L_hdelta` | | H$\delta$ activity index of LRS data ($L_{\rm H\delta}$) |
| `L_hdelta_err` | | uncertainty of $L_{\rm H\delta}$ |
| `M_halpha` | | H$\alpha$ activity index of MRS data ($M_{\rm H\alpha}$) |
| `M_halpha_err` | | uncertainty of $M_{\rm H\alpha}$ |
| `l_halpha` | Å$^{-1}$ | H$\alpha$ absolute flux index of LRS data ($\ell_{\rm H\alpha}$) |
| `l_halpha_err` | Å$^{-1}$ | uncertainty of $\ell_{\rm H\alpha}$ |
| `l_hbeta` | Å$^{-1}$ | H$\beta$ absolute flux index of LRS data ($\ell_{\rm H\beta}$) |
| `l_hbeta_err` | Å$^{-1}$ | uncertainty of $\ell_{\rm H\beta}$ |
| `l_hgamma` | Å$^{-1}$ | H$\gamma$ absolute flux index of LRS data ($\ell_{\rm H\gamma}$) |
| `l_hgamma_err` | Å$^{-1}$ | uncertainty of $\ell_{\rm H\gamma}$ |
| `l_hdelta` | Å$^{-1}$ | H$\delta$ absolute flux index of LRS data ($\ell_{\rm H\delta}$) |
| `l_hdelta_err` | Å$^{-1}$ | uncertainty of $\ell_{\rm H\delta}$ |
| `m_halpha` | Å$^{-1}$ | H$\alpha$ absolute flux index of MRS data ($m_{\rm H\alpha}$) |
| `m_halpha_err` | Å$^{-1}$ | uncertainty of $m_{\rm H\alpha}$ |

Note:
(1) Catalog is stored as `Balmer_line_indexes_stellar_source_catalog_LAMOST_DR9.csv` in the online dataset.
(2) Observational and spectroscopic parameters are from LAMOST DR9 v2.0; if a stellar source was observed multiple times, the medians of the multiple observations are used.
(3) Unavailable values are marked as −9999.0.
